# Supplementary material for: How to Evaluate When You Don't Know How to Evaluate? Choosing Reliable Setups for Base Language Model Benchmarking
Source: arXiv:2610.19185 source file (2026-10-13)
Supplement: Supplementary file 1 [file appendix_picks_generation.tex]

\begin{tabular}{@{}ll@{\hspace{6pt}}ccc@{}}
\toprule
 & & \multicolumn{3}{c}{Norwegian} \\
\cmidrule(lr){3-5}
 & & B & O & W \\
\midrule
Shots & 2B & 5 & 5 & 5 \\
 & Larger & 5 & 5 & 5 \\
\addlinespace[2pt]
Prompts & 2B & sgl & sgl & \textbf{mean} \\
 & Larger & \cellcolor{gray!22}mean & \textbf{sgl} & \cellcolor{gray!22}\textbf{max} \\
\addlinespace[2pt]
Rescaling & 2B & mm & \textbf{z} & \textbf{z} \\
 & Larger & \cellcolor{gray!22}none & \cellcolor{gray!22}\textbf{base} & \cellcolor{gray!22}\textbf{mm} \\
\addlinespace[2pt]
Task agg. & 2B & cat & cat & cat \\
 & Larger & \cellcolor{gray!22}mean & \cellcolor{gray!22}mean & \cellcolor{gray!22}mean \\
\bottomrule
\end{tabular}
